# Supplementary material for: Finite temperature effects on the structural stability of Si-doped HfO$_{2}$ using first-principles calculations
Source: arXiv:2303.14891 ancillary file (2023-03-27)
Supplement: Supplementary file 1 [file suppl_hfsio2.pdf]

# Supplemental Material to "Finite temperature effects on the structural stability of Si-doped $HfO_2$ using first-principles calculations"

Y. Harashima*
*Division of Materials Science, Nara Institute of Science and Technology, Ikoma 630-0192, Japan and Center for Computational Sciences, University of Tsukuba, Tsukuba 305-8577, Japan*

H. Koga, T. Yonehara, and M. Katouda
*Department of Computational Science and Technology, Research Organization for Information Science and Technology, Tokyo 105-0013, Japan*

Z. Ni and H. Matsui
*S-Technology Development Center, Tokyo Electron Technology Solutions Ltd.*

A. Notake and T. Moriya
*Advanced Data Planning Department, Tokyo Electron Ltd.*

M. K. Si and Y. Shigeta
*Center for Computational Sciences, University of Tsukuba, Tsukuba 305-8577, Japan*

R. Hasunuma and A. Uedono
*Faculty of Pure and Applied Science, University of Tsukuba, Tsukuba 305-8573, Japan*

(Dated: March 20, 2023)

This document provides the calculated volumes $V_0$, bulk moduli of zero pressure $B_0$, and the first derivatives of bulk moduli $B_0'$ used in calculations of the Murnaghan equation of states (Eq. (23)). Those values were determined by fitting Eq. (24) using the calculated energies.

TABLE SI. Values of $V_0$ [Å$^3$], $B_0$ [GPa] and $B_0'$ for pristine $HfO_2$ having a tetragonal structure.

| | |
|---|---|
| $V_0$ | 134.6 |
| $B_0$ | 173.1 |
| $B_0'$ | 7.772 |

TABLE SII. Values of $V_0$ [Å$^3$], $B_0$ [GPa] and $B_0'$ for pristine $HfO_2$ having a monoclinic structure.

| | |
|---|---|
| $V_0$ | 140.1 |
| $B_0$ | 186.2 |
| $B_0'$ | 2.026 |

TABLE SIII. Values of $V_0$ [Å$^3$], $B_0$ [GPa] and $B_0'$ for 3% Si-doped $HfO_2$ having a tetragonal structure. In this case, there is only one impurity configuration.

| | 1 |
|---|---|
| $V_0$ | 134.9 |
| $B_0$ | 158.3 |
| $B_0'$ | 5.946 |

TABLE SIV. Values of $V_0$ [Å$^3$], $B_0$ [GPa] and $B_0'$ for 3% Si-doped $HfO_2$ having a monoclinic structure. In this case, there is only one impurity configuration.

| | 1 |
|---|---|
| $V_0$ | 139.5 |
| $B_0$ | 178.7 |
| $B_0'$ | 0.784 |

TABLE SV. Values of $V_0$ [Å$^3$], $B_0$ [GPa] and $B_0'$ for 6% Si-doped $HfO_2$ having a tetragonal structure. In this case, there are nine impurity configurations.

| | 1 | 2 | 3 | 4 | 5 | 6 | 7 | 8 | 9 |
|---|---|---|---|---|---|---|---|---|---|
| $V_0$ | 134.4 | 135.0 | 132.1 | 134.6 | 133.1 | 134.6 | 134.8 | 133.1 | 135.1 |
| $B_0$ | 156.3 | 165.7 | 205.4 | 127.3 | 160.1 | 161.2 | 145.0 | 179.2 | 162.9 |
| $B_0'$ | 9.514 | 7.022 | 6.467 | 23.129 | 11.474 | 9.698 | 0.995 | 6.354 | 3.559 |

TABLE SVI. Values of $V_0$ [Å$^3$], $B_0$ [GPa] and $B_0'$ for 6% Si-doped $HfO_2$ having a monoclinic structure. In this case, there are 23 impurity configurations.

| | 1 | 2 | 3 | 4 | 5 | 6 | 7 | 8 | 9 | 10 | 11 | 12 | 13 | 14 | 15 | 16 | 17 | 18 | 19 | 20 | 21 | 22 | 23 |
|---|---|---|---|---|---|---|---|---|---|---|---|---|---|---|---|---|---|---|---|---|---|---|---|
| $V_0$ | 138.6 | 138.5 | 139.1 | 139.4 | 138.9 | 139.0 | 138.8 | 139.0 | 138.9 | 138.9 | 138.7 | 139.0 | 139.2 | 139.0 | 138.9 | 138.7 | 138.8 | 138.9 | 139.0 | 138.6 | 138.7 | 138.9 | 139.0 |
| $B_0$ | 174.1 | 176.6 | 174.8 | 194.1 | 170.9 | 169.3 | 161.5 | 161.1 | 180.2 | 183.1 | 172.8 | 169.4 | 172.3 | 171.0 | 171.1 | 172.4 | 164.3 | 160.4 | 177.8 | 165.5 | 174.8 | 174.6 | 164.8 |
| $B_0'$ | 3.408 | 2.592 | 4.379 | 1.001 | 4.264 | 4.535 | 7.027 | 6.698 | 4.891 | 5.483 | 6.122 | 3.956 | 4.785 | 3.830 | 4.474 | 6.033 | 5.554 | 5.710 | 3.170 | 6.232 | 3.929 | 3.869 | 4.343 |
